# Supplementary material for: MovieCuts: A New Dataset and Benchmark for Cut Type Recognition
Source: arXiv:2109.05569 source file (2022-10-24)
Supplement: Supplementary file 1 [file pr_curves.tex]

\begin{figure}
\centering
    \includegraphics[width=1\linewidth]
     {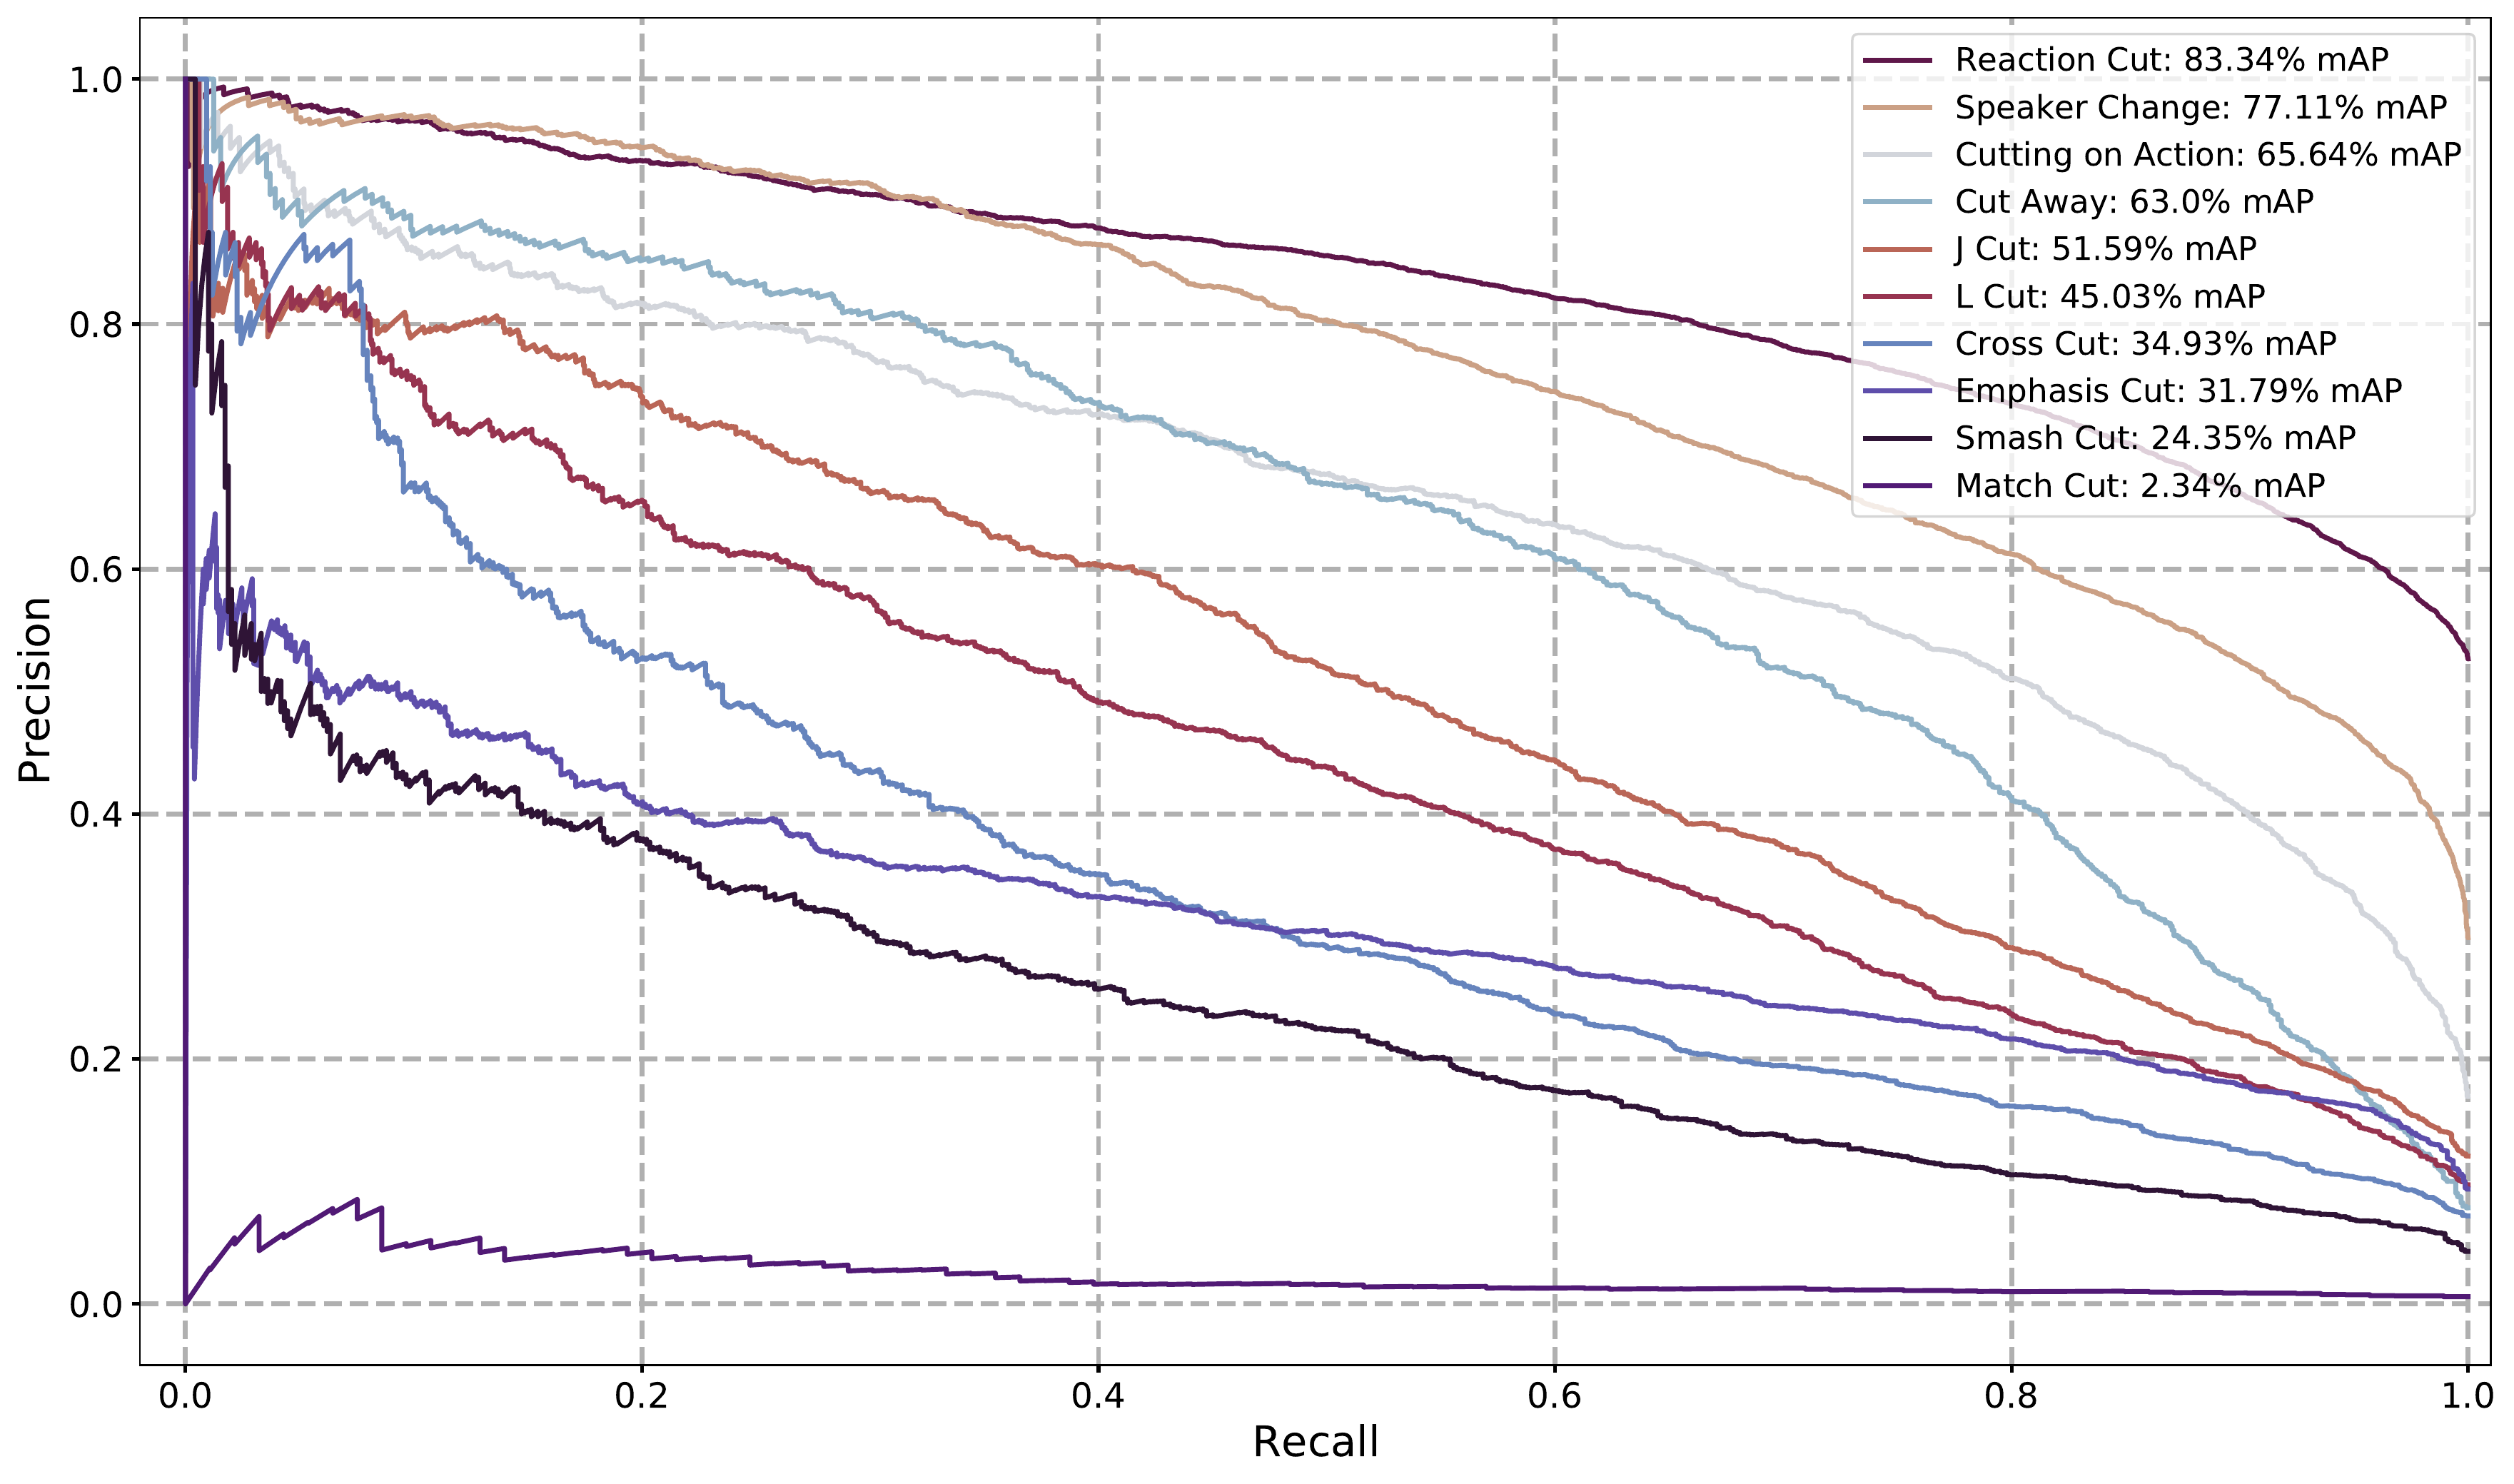}
    \caption{\textbf{Precision vs Recall.} AV + Scaled GB on validation set.}
    \label{figure:pr}
\end{figure}
