# Supplementary material for: MovieCuts: A New Dataset and Benchmark for Cut Type Recognition
Source: arXiv:2109.05569 source file (2022-10-24)
Supplement: Supplementary file 2 [file summary_counts.tex]

\begin{figure}
\centering
    \includegraphics[width=0.95\linewidth]
     {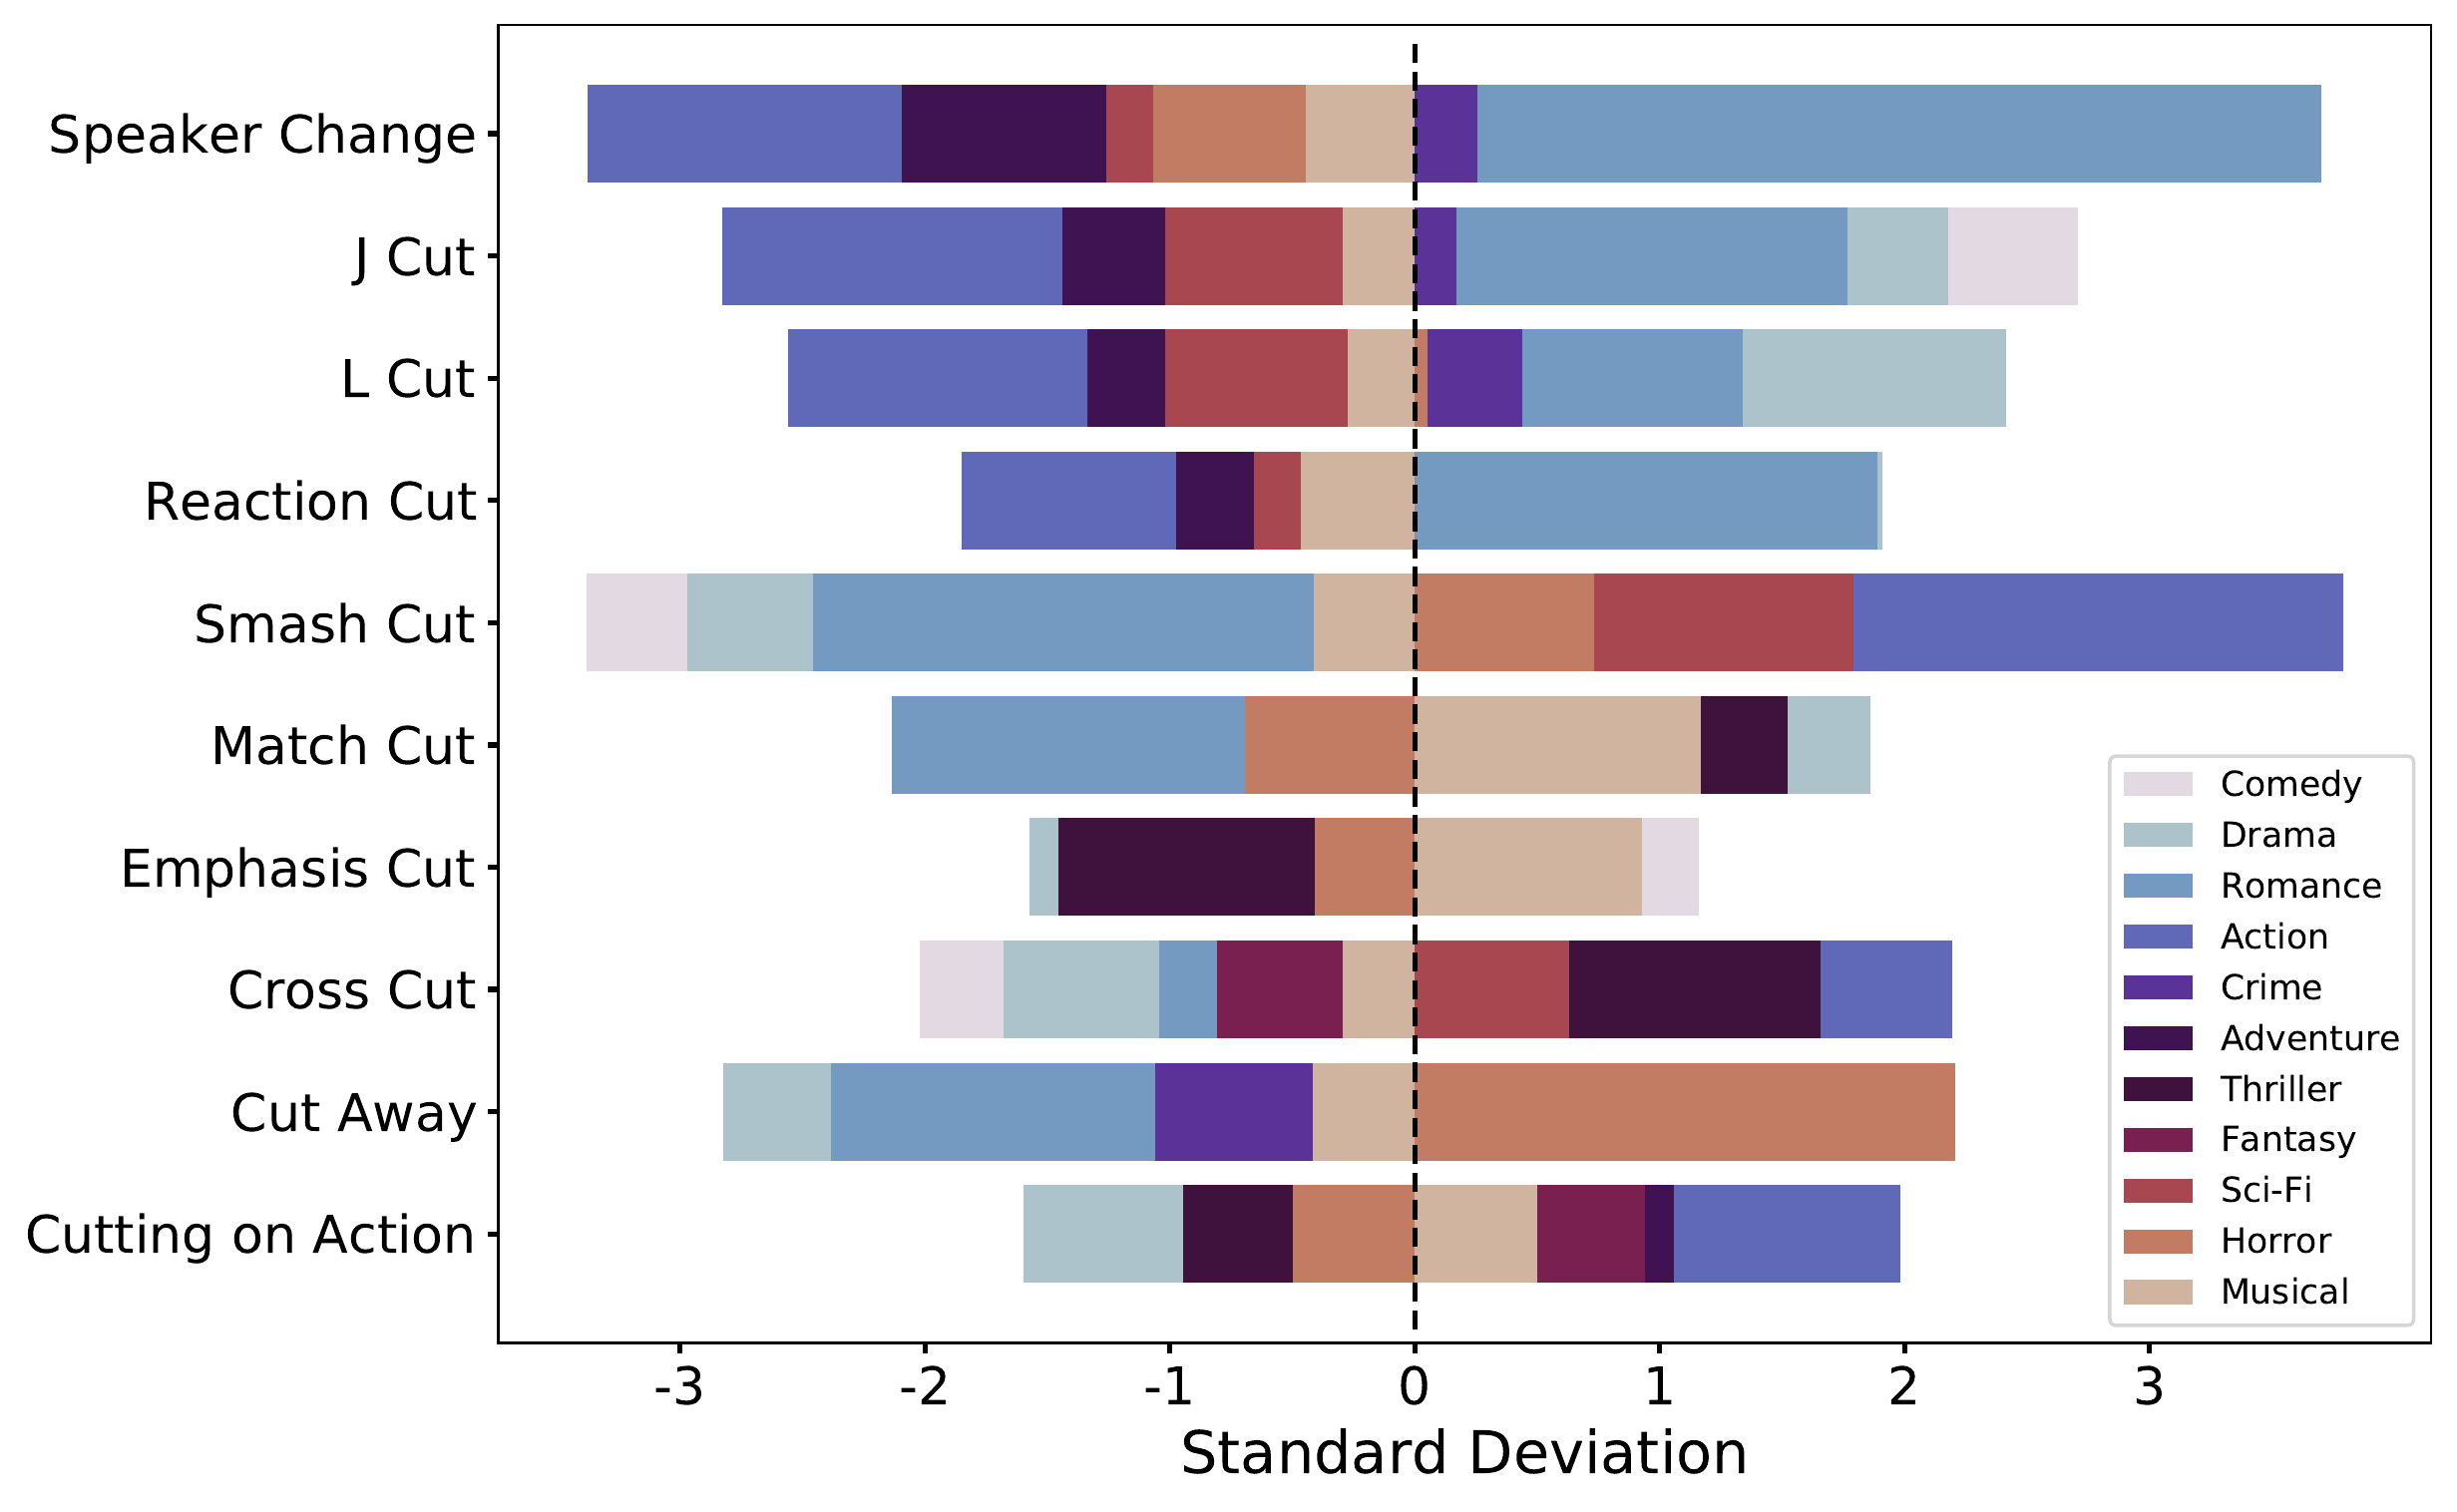}
    \caption{\textbf{Summary of the cut-types' distribution per genre.}}
    \label{figure:summary-counts}
\end{figure}
